# Supplementary material for: Hypergraph Contrastive Collaborative Filtering
Source: arXiv:2204.12200 source file (2022-04-27)
Supplement: Supplementary file 1 [file appendix.tex]

\section{Appendix}
\label{sec:appendix}
